# Supplementary material for: Semi-automatic selection of summary statistics for ABC model choice
Source: arXiv:1302.5624 ancillary file (2013-02-22)
Supplement: Supplementary file 1 [file supplement.pdf]

# Supplementary Material for Semi-automatic selection of summary statistics for ABC model choice

Dennis Prangle*†, Paul Fearnhead†, Murray P Cox‡§, Patrick J Biggs‡¶ and Nigel P French‡¶

## 1 Asymptotic Monte Carlo error for ABC model choice

As described in the main text, approximation errors enter ABC results through (i) non-sufficient summary statistics (ii) the effect of $h$ on the ABC target distributions $p_{\text{ABC}}$ and $\pi_{\text{ABC}}$ and (iii) the Monte Carlo approximations of $p_{\text{ABC}}$ and $\pi_{\text{ABC}}$ from a finite sample. Reducing $h$ decreases error due to (ii) but increases that from (iii). A curse of dimensionality result shows that the rate of this latter increase rises with the dimension of $S$, motivating selection of low dimensional summary statistics. This section recaps relevant results on this from Fearnhead and Prangle (2012) and confirms they apply in the model choice setting.

*d.prangle@lancaster.ac.uk
†Department of Mathematics and Statistics, Lancaster University, UK
‡Allan Wilson Centre for Molecular Ecology and Evolution, Massey University, Palmerston North, New Zealand
§Institute of Fundamental Sciences, Massey University, Palmerston North, New Zealand
¶Infectious Disease Research Centre, Institute of Veterinary, Animal and Biomedical Sciences, Massey University, Palmerston North, New Zealand

Output from an ABC rejection sampling algorithm similar to Algorithm 1 in the main paper can be used to make the following estimate of $\Pr(\mathcal{M}_i|S(x_{\text{obs}}))$:

$$\hat{q}_i = N_{\text{acc}}^{-1} \sum_{j=1}^{N_{\text{acc}}} \mathbb{I}(\mathcal{M}_j^* = \mathcal{M}_i),$$

where $N_{\text{acc}}$ is the size of the accepted sample. That is, $\hat{q}_i$ is the proportion of acceptances from the model of interest. (For Algorithm 2, to get probability estimates the $\hat{q}_i$ values must be reweighted by the prior model weights, but their properties are still crucial to the algorithm's performance.) The asymptotic variance of $\hat{q}_i$ for a large number of proposals $N$ is

$$\mu_i(1 - \mu_i)/E[N_{\text{acc}}]$$

where $\mu_i = p_{\text{ABC}}(\mathcal{M}_i|S(x_{\text{obs}}))$, the probability of $\mathcal{M}_i$ under the ABC target distribution. (For Algorithm 2, instead $\mu_i \propto p_{\text{ABC}}(\mathcal{M}_i|S(x_{\text{obs}})/p_M(\mathcal{M}_i).)$ Lemma 1 of Fearnhead and Prangle (2012) gives an asymptotic expression for the probability of acceptance in an iteration of the algorithm for small $h$,

$$E[N_{\text{acc}}]/N = \pi(S(x_{\text{obs}}))h^d + o(h^d),$$

where $d = \dim(S)$ and $\pi(S(x_{\text{obs}}))$ is the prior predictive density of the observed summary statistics. The proof of this lemma in Fearnhead and Prangle (2012) for the case of a single model immediately extends to multiple models (by taking expectations with respect to $(\mathcal{M}, \theta)$ rather than $\theta$.)

This shows that in a rejection sampling algorithm, the asymptotic rate of convergence of an estimated ABC model weight to $\Pr(\mathcal{M}_i|S(x_{\text{obs}}))$ reduces as $\dim(S)$ is increased. Arguments in Appendix A of Fearnhead and Prangle (2012) also show that a similar effect typically occurs for an importance sampling or sequential Monte Carlo (SMC) algorithm. As SMC involves importance sampling steps, the key part of the

argument is to establish that the effective sample size of ABC importance sampling crucially depends on the quantity $E[N_{\mathrm{acc}}]/N$ discussed above. Fearnhead and Prangle (2012) give the details for the case of a single model and they extend easily to multiple models by adjusting how expectations are taken as described above.

## 2 Details of SMC algorithm

This section describes an SMC ABC algorithm, essentially that of Toni and Stumpf (2010), which is used for the analysis of *C. jejuni* data in the main text. Following the algorithm is a description of the tuning choices used for this analysis.

**Notation** Models are denoted here by an indicator $m \in \{1, 2, \ldots, M\}$. The $t$th weighted particle estimate is defined by model indicators $m_i^{(t)}$, parameters vectors $\theta_i^{(t)}$ and weights $w_i^{(t)}$ for $1 \leq i \leq N$.

**Input**

Model prior $p_M(m)$.

Parameter priors $\pi(\theta|m)$ for each $m \in \{1, 2, \ldots, M\}$.

Algorithm to simulate from $x|m, \theta$.

A summary statistics function $S(\cdot)$.

Observed summary statistics $s_{\text{obs}}$.

Distance function $d(\cdot, \cdot)$.

Swap probability $\alpha$.

Number of particles $N$.

Rule to choose model update kernels $K^{(t)}(\cdot|m)$.

Rule to choose parameter update kernels $K^{(t)}(\cdot|\theta, m)$.

Initial threshold $h_1$.

Stopping condition (see step 4).

Rule to choose new thresholds (see step 5).

**Algorithm**

1 Initialise threshold counter $t = 1$.

2 Loop over $i = 1, 2, \ldots, N$.

2.1 If $t = 1$:

2.2 Sample $m^{**}$ from $p_M(m)$.

2.3 Sample $\theta^{**}$ from $\pi(\theta|m = m^{**})$.

2.4 Else:

2.5 Sample $j$ from $1, 2, \ldots, N$ with $\Pr(j) = w_j^{(t-1)}$. Let $m^* = m_j^{(t-1)}$.

2.6 With probability $\alpha$ sample $m^{**}$ from $K^{(t)}(m^{**}|m^*)$. Otherwise let $m^{**} = m^*$.

2.7 Sample $j$ from $1, 2, \ldots, N$ with $\Pr(j) \propto w_j^{(t-1)} \mathbb{I}(m_j^{(t-1)} = m^{**})$. Let $\theta^* = \theta_j^{(t-1)}$.

2.8 Sample $\theta^{**}$ from $K^{(t)}(\theta^{**}|\theta^*, m^{**})$.

2.9 If $p_M(m^{**})\pi(\theta^{**}|m = m^{**}) = 0$ return to step 2.5.

2.10 Simulate data $x^*$ conditional on $(m^{**}, \theta^{**})$ and compute $s^* = S(x^*)$.

2.11 If $d(s_{\text{obs}}, s^*) > h_t$ return to step 2.1.

2.12 Set $m_i^{(t)} = m^{**}$, $\theta_i^{(t)} = \theta^{**}$ and

$$w_i = \begin{cases} 1 & \text{if } t = 1 \\ p_M(m^{**})\pi(\theta^{**}|m^{**})/(S_1 S_2) & \text{otherwise,} \end{cases}$$

where $S_1 = (1-\alpha) \sum_{i|m_i^{(t-1)}=m^{**}} w_i^{(t-1)} + \alpha \sum_{i|m_i^{(t-1)}\neq m^{**}} w_i^{(t-1)} K^{(t)}(m^{**}|m_i^{(t-1)})$

and $S_2 = \dfrac{\sum_{i|m_i^{(t-1)}=m^{**}} w_i^{(t-1)} K^{(t)}(\theta^{**}|\theta_i^{(t-1)}, m^{**})}{\sum_{i|m_i^{(t-1)}=m^{**}} w_i^{(t-1)}}$.

2.13 End loop.

3 Let $w_i^{(t)} = w_i / \sum_{i=1}^N w_i$ for $1 \leq i \leq N$.

4 End algorithm if stopping condition reached.

5 Increment $t$ by 1, calculate $h_t$ and return to step 2.

**Tuning choices** The *C. jejuni* application in the main paper used $\alpha = 0.1$ and $N = 1000$. The main text details the choice of $d(\cdot, \cdot)$, stopping condition and rule to update the threshold. The model update kernel $K^{(t)}(\cdot, m)$ places equal weight on all models $k \neq m$ such that $\sum_{i|m_i^{(t-1)}=k} w_i^{(t-1)} > 0$. The parameter update kernel

$K^{(t)}(\cdot|\theta, m)$ is the density of $N(\theta, 2\Lambda_m^{(t)})$ where $\Lambda_m^{(t)}$ is a diagonal matrix composed of sample variances of the parameters conditional on model $m$ calculated from the $t-1$th particle estimate. This choice follows Beaumont et al. (2009).

# 3 Genetic summaries

The section details the genetic summaries of a MLST dataset used in the *C. jejuni* application. There are two groups, summaries of the entire data, and summaries relating to a single locus. Summaries which are starred are those used in the pilot analysis. To keep $\dim(S)$ reasonably low in the pilot, starred entries in the locus summaries were summarised by the mean and variance over all seven loci. For the main analysis, summaries for every locus were used as regression covariates. We considered two ways to order these: by locus identity, or by magnitude. Both orderings were used, so each locus summary listed below contributes 14 summaries. This gives a total of 15 statistics used in the pilot and 125 used as regression covariates.

**Global summaries**

**Single locus variants (SLVs)*** The number of unordered pairs of isolates in which exactly one allele differs (Feil et al., 2004).

**Mean SLV site differences*** For any pair of isolates the number of nucleotides which differ can be calculated. This number is calculated for every pair of isolates in which exactly one allele differs (i.e. those which are counted as an SLV), and the mean of these values taken.

**Unique sequence types (STs)*** The number of unique STs within the dataset.

**Max ST frequency*** The maximum frequency of any ST in the dataset.

**Mean ST frequency*** The mean frequency of all STs in the dataset.

**Mean allele differences*** For any pair of isolates the number of alleles which differ can be calculated. This is calculated for every unordered pair of isolates and the mean taken.

**ST heterozygosity** A heterozygosity-like summary of ST frequencies $u_1, \ldots, u_d$: $1 - \sum_{i=1}^{d} u_i^2$.

**ST entropy** Shannon entropy of ST frequencies: $\sum_{i=1}^{d} u_i \log u_i$.

**STs with frequency 1/2/3/4/$>$ 4** The number of STs with the given frequency.

**Locus summaries**

**Segregating sites*** The number of nucleotides which are not constant for all alleles.

**Mean site differences*** For any pair of isolates the number of nucleotides in the locus of interest which differ can be calculated. This is calculated for every unordered pair of isolates and the mean taken, as in Tajima (1983).

**Number of alleles*** The number of unique alleles.

**Maximum allele frequency*** The maximum frequency of any allele.

**Mean allele frequency*** The mean frequency of all alleles.

**Allele heterozygosity** A heterozygosity-like summary of allele frequencies $v_1, \ldots, v_d$: $1 - \sum_{i=1}^{d} v_i^2$.

**Allele entropy** Shannon entropy measure of allele frequencies: $\sum_{i=1}^{d} v_i \log v_i$.

**Linkage disequilibrium*** This is based on the Hedrick (1987) $D'$ summary of linkage disequilibrium between a pair of loci. The statistic used is the mean of $D'$ values between the locus of interest and the others.

# 4 Marginal parameter posteriors

Figures 1 and 2 show estimated marginal parameter posteriors of the *C. jejuni* analyses from the main text. These show that: recombination rate estimates are low in comparison with the prior; little is learnt about mean track length; the mutation rate estimate under the main analysis is more concentrated than the prior; relative growth estimates concentrate on small values in comparison with the prior, especially under the main analysis.

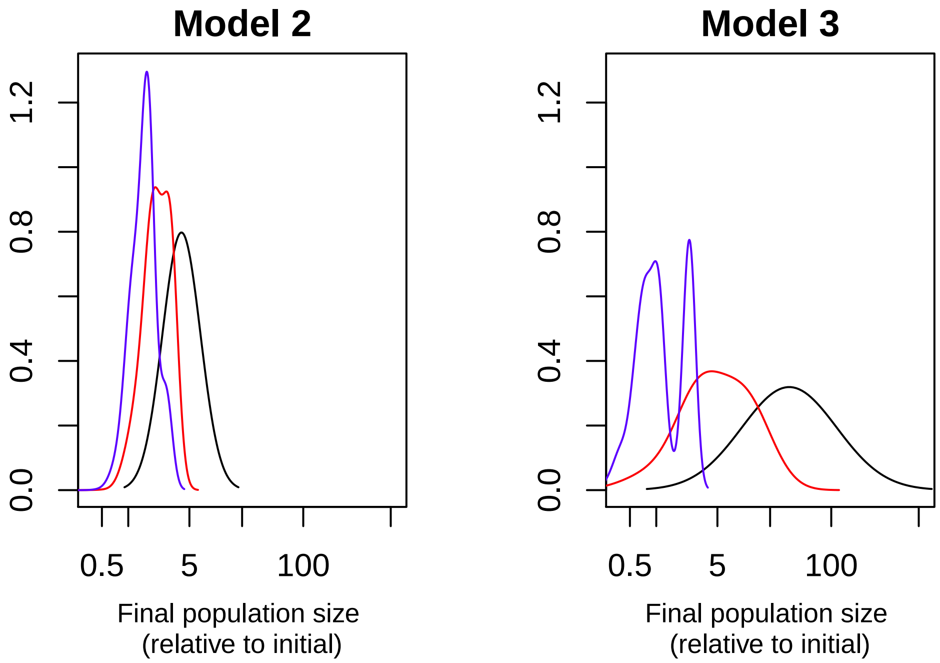


Figure 1: Kernel density estimates of marginal posteriors for the growth parameter (i.e. ratio of final population size to initial population size), from analysis of *C. jejuni* data. Weighted density estimates were formed from ABC output from the pilot (red) and main (blue) analyses. Prior densities are also shown (black). The graphs show results conditional on the 2 models allowing growth. The density estimates were computed and plotted on a log scale, but the x-axes are labelled in the original units for ease of interpretation.

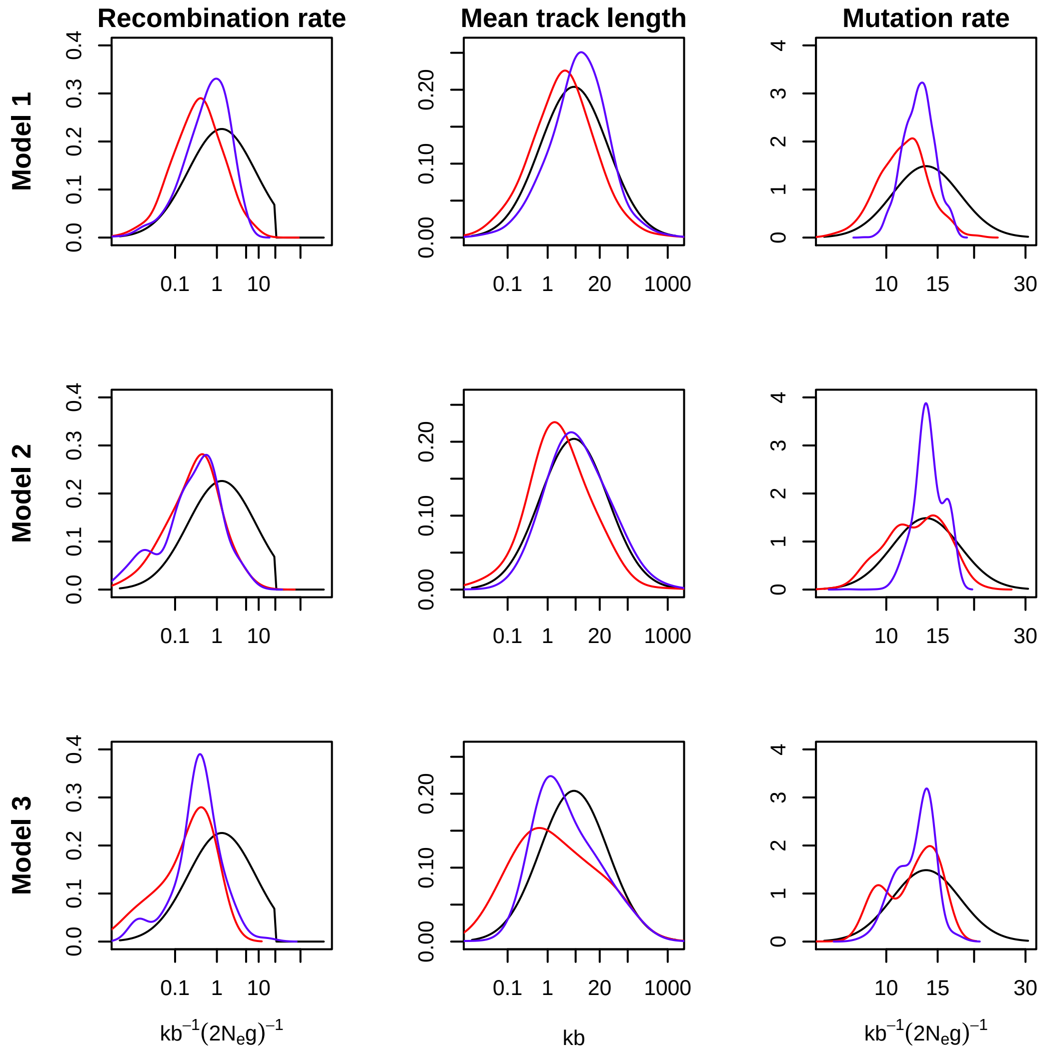


Figure 2: Kernel density estimates of marginal parameter posteriors, excluding relative growth, from analysis of *C. jejuni* data. Weighted density estimates were formed from ABC output from the pilot (red) and main (blue) analyses. Prior densities are also shown (black). The rows represent output conditional on the 3 different models, and the columns different parameters. The density estimates were computed and plotted on a log scale, but the x-axes are labelled in the original units for ease of interpretation.

# 5 Influence of genetic summaries on the pilot analysis

Output of the pilot analysis of *C. jejuni* data was used to perform a detailed investigation of the qualitative fit of the models to the data, as follows. The SMC algorithm provides weights for each $(\mathcal{M}, \theta, S(x))$ output triple. Following Ratmann et al. (2009), we summarise the resulting marginal distributions of each component of $S$ in Figure 3. Note that models 2 and 3 produced small effective sample sizes, so their distributions, particularly the extremes, are less well estimated. Nonetheless, the results show that several statistics were hard to fit for models 2 and 3. In particular, the number of mean SLV site differences was hard to fit under any model – only four simulations were above the observed value, all produced by model 1. To determine whether fitting this particular statistic dominated the results, we reran the pilot analysis without it and found similar results (model 1 85%, model 2 8%, model 3 6%). Models 2 and 3 also poorly fitted the mean frequency of sequence types and number of unique sequence types. Finally, all models tended to produce more SLVs than the observed data, which may indicate model misspecifation.

A similar investigation was attempted for the main analysis. Here it was only possible to consider the fits of the 7 summary statistics produced by fitting regressions. No interesting results were found; all models were capable of producing each observed summary statistic.

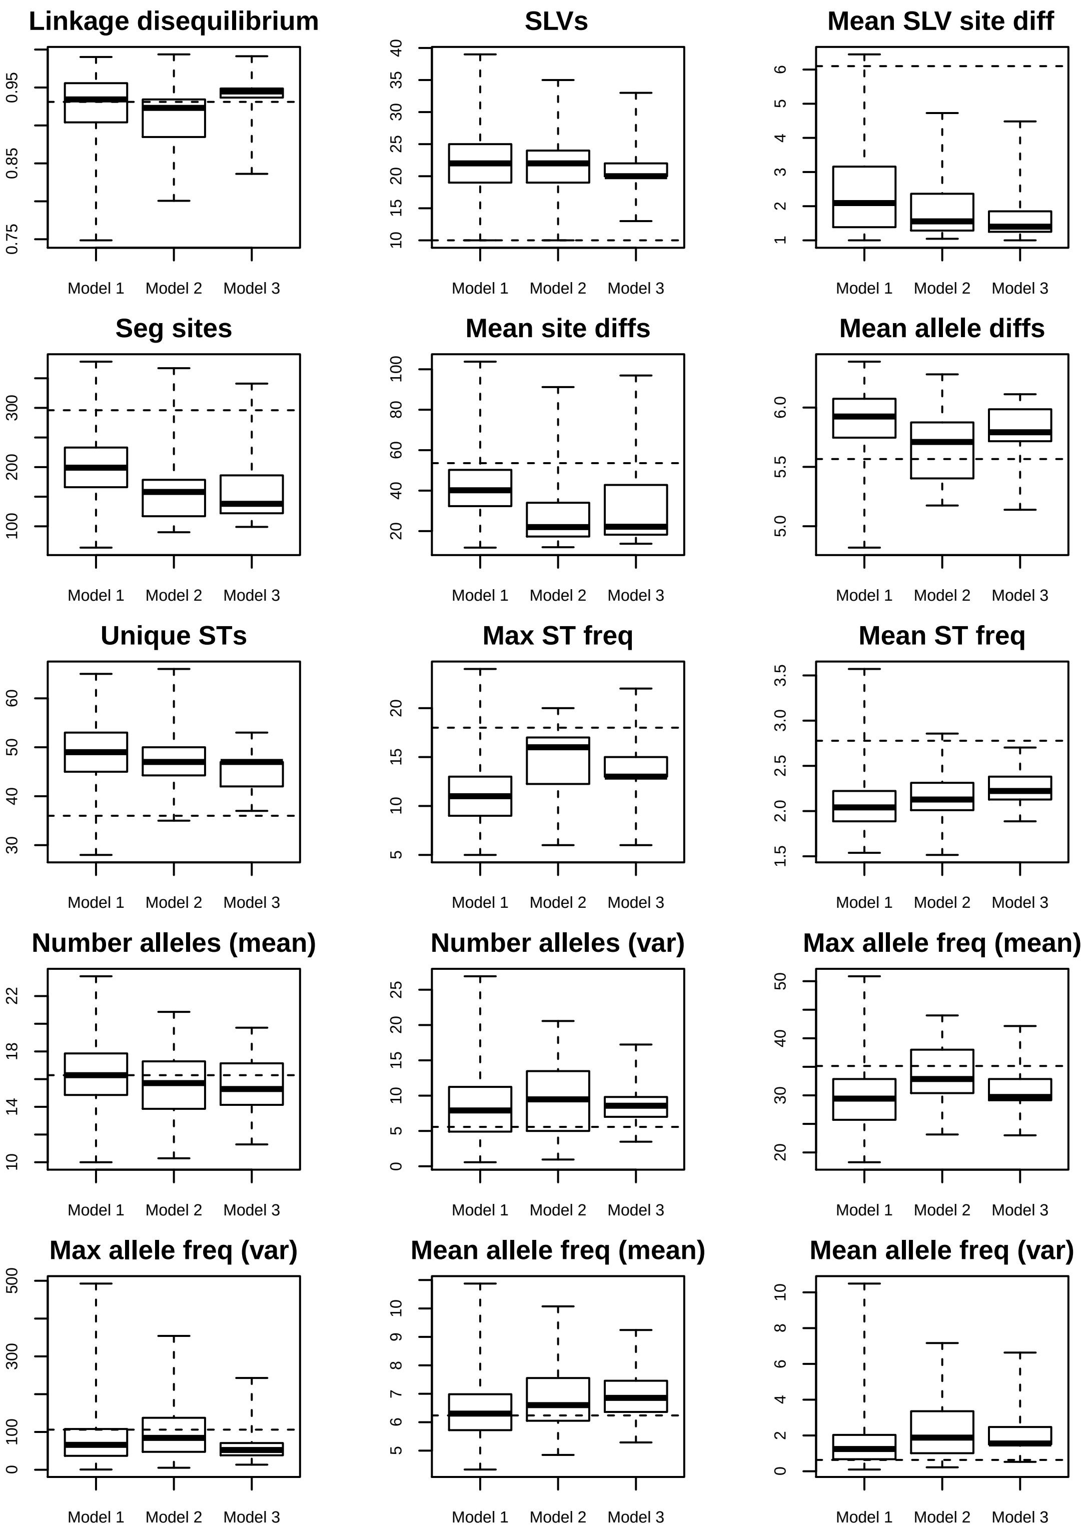


Figure 3: Marginal distributions of summary statistics from the pilot analysis output. The box plots show quartiles computed from weighted samples. Horizontal lines show the observed summary statistics.

# 6 Structure of fitted regressions

This section assesses the informativeness of the genetic summaries to the regressions used in the *C. jejuni* analysis.

**Methods** A crude assessment of informativeness of covariates can be made from their influence on the fitted predictors, as follows. Consider first a general fitted linear regression $\hat{\theta} = a + \sum_{j=1}^{p} b_j x_j$. A measure of the influence of the $j$th covariate is $b_j (\mathrm{Var}\, x_j)^{1/2}$, the regression coefficient of the normalised covariate $x_j / (\mathrm{Var}\, x_j)^{1/2}$.

Recall that each of our summary statistics is of the form $S_i(x) = h_i(\beta_i^T f_i(x))$. We can write the linear combination as

$$\beta_i^T f_i(x) = \sum_{j=1}^{p} \sum_{k=1}^{3} \beta_{ijk} g_{ijk}(t_j(x)),$$

where $t_j(x)$ is the $j$th genetic summary, and $g_{ij1}, g_{ij2}, g_{ij3}$ are three spline basis functions calculated for $t_j(x)$ from the simulated data (The dependence on $i$ is because this can determine which simulated data is used.) Let

$$\alpha_{ij} = \max_k |\beta_{ijk} [\mathrm{Var}\, g_{ijk}(t_j(x))]^{1/2}|,$$

where sample variance over the relevant training data is used. The $\alpha_{ij}$ value is the maximum in magnitude of the coefficients for the normalised functions of summary $t_j$. In this section we report a relative informativeness statistic,

$$\alpha'_{ij} = 100 \alpha_{ij} / \max_j \alpha_{ij}.$$

The $\alpha'$ statistic is used to report the most informative genetic summaries for each regression in Table 1, and mean informativeness values in Table 2. Table 1 also reports an estimate of the quality of out-of-sample fit for each regression, based on

cross-validation. For the four continuous parameters this is a root mean squared standardised error (RMSSE) i.e. root mean squared error of responses standardised to have variance 1. Standardisation allows comparison of the relative quality of the regressions. A constant estimate of the parameter mean would achieve 1. For model choice the deviance is given i.e. $-2$ times the log of the expected likelihood contribution for a single new observation. Here 0 equates to perfect prediction and $-2 \log 0.5 \approx 1.39$ to always predicting equal model weights.

**Results** Tables 1 and 2 show that genetic summaries involving counting nucleotide differences are the most informative overall and for each individual regression except mean track length. In particular, the largest in magnitude of the mean site difference values for individual loci had an $\alpha'$ value nearly twice that of the next statistic in 3 regressions. Also of interest is that the regressions targeting the growth parameter and distinguishing betwen models 2 and 3 were the least informative, while targeting the distinction between a growth and non-growth model was more successful.

| Target | RMSSE | Deviance | Genetic summary | $\alpha'$ |
|---|---|---|---|---|
| Recombination rate | 0.64 | | Mean SLV site difference | 100 |
| | | | Linkage disequilibrium (glyA 4) | 69 |
| | | | Segregating sites (magnitude 1) | 67 |
| | | | Linkage disequilibrium (gltA 3) | 57 |
| | | | Segregating sites (magnitude 2) | 56 |
| Mean track length | 0.69 | | Linkage disequilibrium (uncA 7) | 100 |
| | | | Linkage disequilibrium (aspA 1) | 94 |
| | | | Mean SLV site difference | 55 |
| Mutation rate | 0.60 | | Mean site differences (magnitude 1) | 100 |
| | | | Mean site differences (magnitude 2) | 99 |
| | | | Mean SLV site differences | 68 |
| | | | Segregating sites (magnitude 6) | 65 |
| | | | Mean site differences (magnitude 4) | 64 |
| | | | Segregating sites (magnitude 3) | 61 |
| | | | ST heterozygosity | 54 |
| | | | Segregating sites (magnitude 2) | 53 |
| | | | Segregating sites (magnitude 1) | 53 |
| Relative growth | 0.85 | | Mean site differences (magnitude 1) | 100 |
| | | | Mean site differences (magnitude 2) | 59 |
| Model 1/2 | | 0.69 | Segregating sites (magnitude 1) | 100 |
| | | | ST heterozygosity | 86 |
| | | | Mean SLV site differences | 71 |
| | | | Mean site differences (magnitude 4) | 66 |
| | | | Mean freq (magnitude 7) | 50 |
| Model 2/3 | | 1.25 | Mean site differences (magnitude 1) | 100 |
| Model 1/3 | | 0.46 | Mean site differences (magnitude 1) | 100 |
| | | | Segregating sites (magnitude 1) | 59 |
| | | | Mean site differences (magnitude 4) | 54 |
| | | | Mean site differences (magnitude 3) | 52 |

Table 1: Exploratory summaries of regressions used by semi-automatic ABC to fit $S$. A cross-validation estimate of the error is shown for each regression. Also reported are the genetic summaries with largest relative influences $\alpha'$ in each regression. All $\alpha'$ values $> 50$ are reported. Details of the summaries are given in Section 3. For locus based summaries ordered by magnitude, 1 represents the largest magnitude and 7 the smallest.

| Genetic summary group | Mean $\alpha'$ |
|---|---|
| Mean allele differences | 1 |
| Max ST frequency | 2 |
| Mean ST frequency | 5 |
| Linkage disequilibrium (magnitude) | 5 |
| Unique STs | 5 |
| Allele entropy (locus) | 5 |
| Allele heterozygosity (locus) | 5 |
| Max ST frequency | 6 |
| Unique STs | 6 |
| Allele heterozygosity (magnitude) | 6 |
| Number of alleles (magnitude) | 7 |
| Maximum allele frequency (magnitude) | 8 |
| Mean allele frequency (magnitude) | 10 |
| Alleles entropy (magnitude) | 11 |
| Segregating sites (locus) | 11 |
| Number of alleles (locus) | 12 |
| Mean ST frequency | 13 |
| Linkage disequilibrium (locus) | 14 |
| ST entropy | 14 |
| Mean site differences (locus) | 15 |
| SLVs | 19 |
| ST heterozygosity | 20 |
| Segregating sites (magnitude) | 21 |
| Mean site differences (magnitude) | 29 |
| Mean SLV site differences | 54 |

Table 2: Mean relative influence values for each group of genetic summaries as detailed in Section 3. For global summaries, the mean across all regressions is reported. For local summaries, we report two results for each group; one when ordered by locus identity and another for magnitude ordering. In each case we take the mean across all regressions and across each of the 7 summaries in the group.

# 7 Regression modelling choices

This section investigates various choices made in the regressions to produce summary statistics for the *C. jejuni* application. To perform the investigations the method of Section 6.2 in the main text was used to simulate $2 \times 10^4$ data sets from the training region. This was used to investigate the change in regression fit as several modelling choices were varied.

**Number of isolates** Data sets with 200 isolates were simulated, and regressions performed using $f(x)$ calculated from $n = 10, 20, \ldots, 200$ isolates. The regressions and calcuation of $f(x)$ were otherwise performed as in the main text. Figure 4 plots $n$ against cross-validation estimates of the regression error (described in Section 6). Regression error is shown to decrease with $n$, but at a decreasing rate; reduction in error is roughly proportional to increase in $\log n$.

The choice of $n = 100$ in the main text is pragmatic, based on the computing time available. This analysis confirms that gains in regression quality are possible by increasing $n$ but are increasingly costly (as time to simulate a dataset was found to be roughly linear in $n$).

**Pooling** Regression fitting for continuous parameters as described in Section 6.2 of the main text was repeated using a) combined simulated data and b) simulated data from an individual model. As in the main text, combined simulated data means data from all models, except for the growth parameter regression where it is data from all models with growth. Approach b) was performed for each model, with the exception that the growth parameter regression could not be performed for data from the no growth model. For each fitted regression, predictions were computed for all simulated data sets. For every parameter, Pearson correlation coefficients were calculated between each sequence of predicted values. All were above 0.88. This

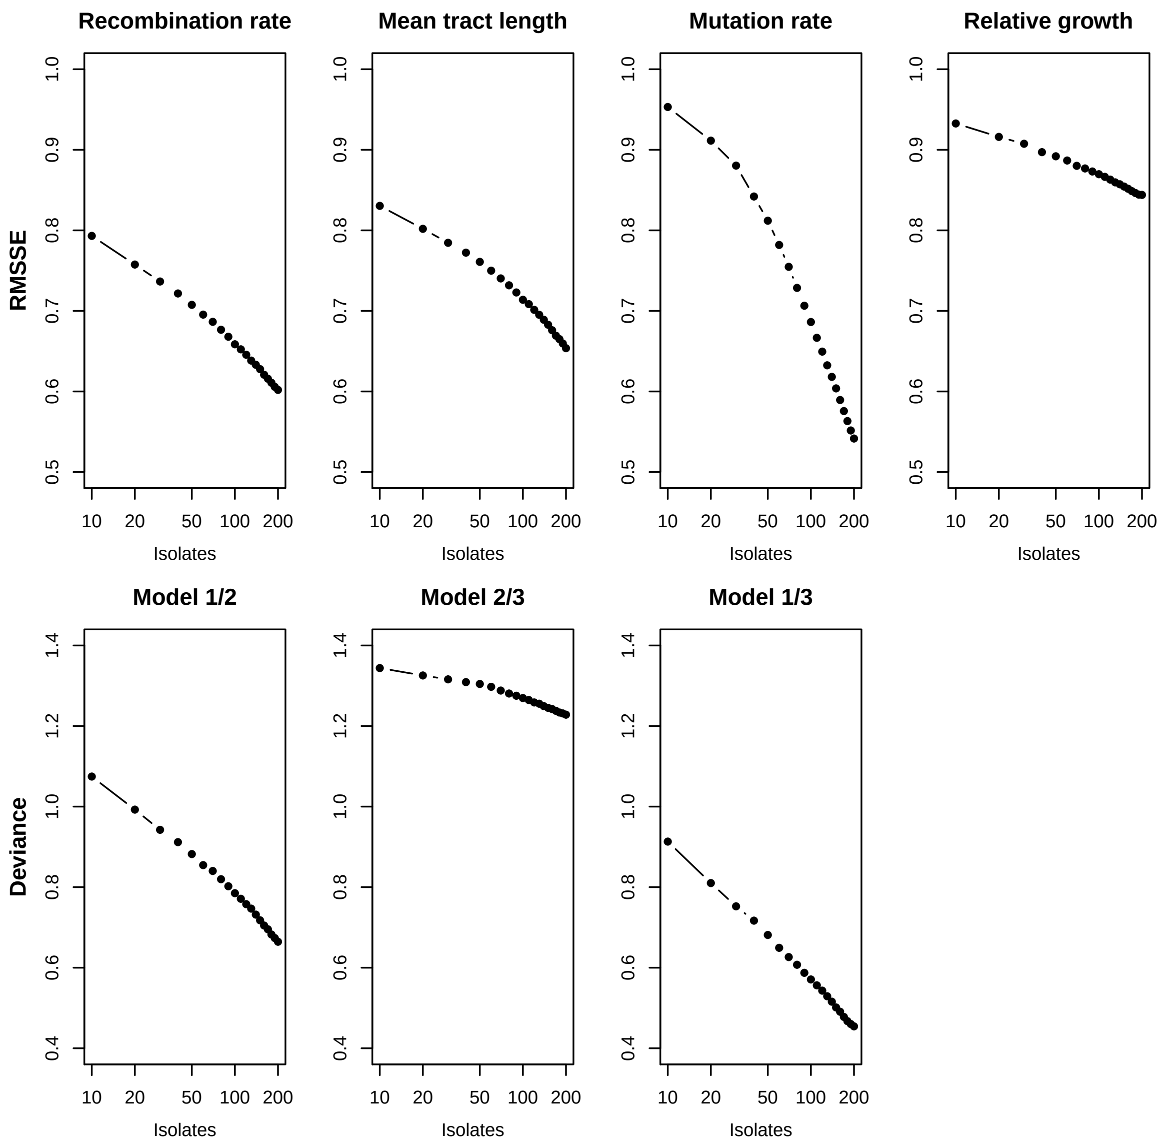


Figure 4: Plots of number of isolates used to create regression covariates against an estimate of the quality of the fit: root mean squared standarised error (RMSSE) for linear regressions, and deviance for logistic regressions. Each plot represents to a different target. The $x$ axis is shown on a log scale.

exploratory analysis shows that for any given parameter the predictions produced by different fitted regressions are close to linear transformations of each other. This suggests they will therefore behave similarly as components of $S$ in an ABC algorithm and justifies using a single parameter estimator for each parameter in $S$ produced via approach a).

**Data transformation** Regression fitting as in the main text was repeated using various choices of data transformation $f(\cdot)$. We considered transformations of the form $f(x) = (1, f_1(x), f_2(x), \ldots, f_n(x))$ which are the concatenation of a constant term and several vectors of transformations. For *polynomial* $f(\cdot)$, $f_i(x)$ is formed by taking element-wise $i$th powers of $x$. For *spline* $f(\cdot)$, a $B$-spline basis of order $n$ is calculated for each component of $x$, with knots given by quantiles of simulated values, and $f_i(x)$ is formed by taking element-wise $i$th basis function values for $x$.

Table 3 shows estimates of the quality of out-of-sample fit based on cross-validation, as in Section 6. The results shows that the final choice of splines with $n = 3$ is close to the best for each regression, although the improvement in fit compared to $f(x) = (1, x)$ is modest.

| $f(\cdot)$ type | $n$ | Recombination rate | Mean tract length | Mutation rate | Relative growth | Model 1/2 | Model 2/3 | Model 1/3 |
|---|---|---|---|---|---|---|---|---|
| Polynomial | 1 | 0.672 | 0.722 | 0.628 | 0.870 | 0.728 | 1.270 | 0.507 |
| Polynomial | 2 | 0.660 | 0.692 | 0.617 | 0.854 | 0.735 | 1.246 | 0.484 |
| Polynomial | 3 | 0.654 | 0.689 | 0.607 | 0.854 | 0.740 | 1.250 | 0.519 |
| Polynomial | 4 | 0.648 | 0.688 | 0.611 | 0.858 | 0.739 | 1.251 | 0.522 |
| Spline | 2 | 0.656 | 0.691 | 0.612 | 0.852 | 0.708 | 1.249 | 0.477 |
| Spline | 3 | 0.638 | 0.681 | 0.609 | 0.848 | 0.703 | 1.243 | 0.472 |
| Spline | 4 | 0.638 | 0.680 | 0.606 | 0.851 | 0.703 | 1.247 | 0.471 |

Table 3: Cross-validation estimates of regression quality for various choices of $f(\cdot)$. For continuous parameters the figures are estimates of root mean squared error of responses standardised to have unit variance. For model choice regressions an estimate of the deviance is given.

# 8 Validation study on simulated data

For the simple examples in Section 5 of the main text, the performance of ABC model choice analyses was validated by analysing 100 data sets simulated from known models. This was not feasible for the *C. jejuni* application due to the larger computational cost of an ABC analysis. Instead a smaller scale study was performed to provide an exploratory test of the method.

We simulated 3 parameter sets from the prior for biological parameters (i.e. all except relative growth) truncated to the training region, and 3 growth parameters for each model similarly. For each of the 9 combinations of biological and demographic parameters a dataset was simulated. ABC analyses of these were performed taking $S$ as in a) the pilot analyses and b) our main analysis. The latter is an approximation of a semi-automatic ABC analysis that avoids the cost of repeating the regression stage of the analysis. We assume this would produce similar results since the training interval for each parameter is wide (in that its prior probability is high). All ABC analyses used 1000 parameters and terminated on the iteration after $4 \times 10^4$ simulations (twice as many iterations as used in the pilot analysis in the main paper). This gives both types of ABC analysis roughly equal computational cost.

Figure 5 shows the model choice results, illustrating that the main analysis distinguishes better between the models. In particular, the no growth model is correctly assigned the majority of the weight for the 3 relevant data sets. Both analyses are less successful at inference for data simulated from a model with growth. In some cases the no growth model is correctly given a very low probability, but the growth models are poorly distinguished.

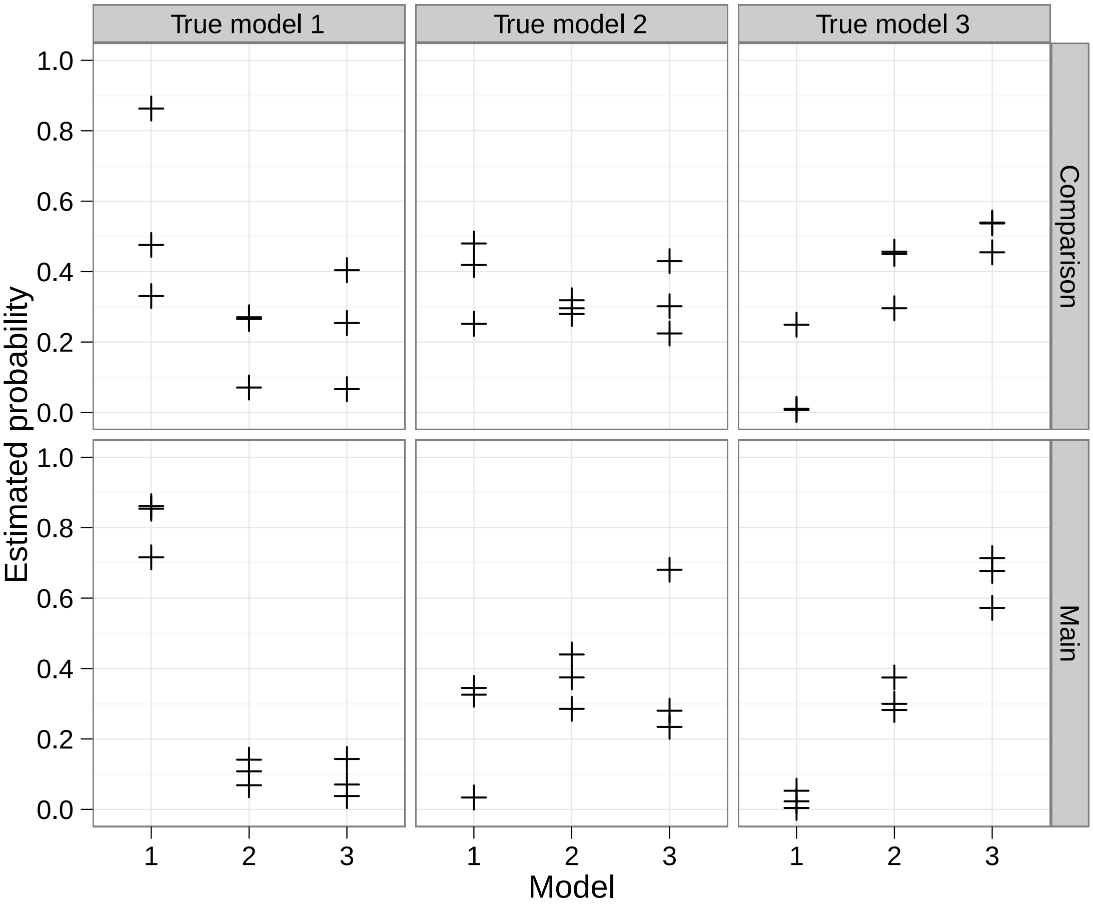


Figure 5: Estimated model probabilities from ABC analyses of 9 simulated data sets. Each data set is analysed by a comparison analysis ($S$ as in the pilot analysis of the main text) and a main analysis ($S$ as in the main analysis of the main text). Rows represent type of analysis and columns which model generated the data.

# 9 Sensitivity analyses

## 9.1 Prior sensitivity

This section performs ABC analyses for the *C. jejuni* application under alternative parameter priors. This investigates whether our model choice results are robust to prior assumptions. The alternative priors considered are summarised in Table 4. The single alternative prior for biological parameters (i.e. all except relative growth) aims at being less informative (labelled as "uninformative" in tables below, which used in a relative sense only) while avoiding placing weight on parameter values which cause long simulation times. We consider two alternative demographic priors. The first gives both growth models equal prior relative growth variance, and the second has equal relative growth priors, leaving the start date of growth as the only difference. These investigate the relative effects of the growth prior and start date of growth on the results. There are a total of 6 combinations for the prior, including that used in the main paper.

| Parameter | Units | Model | Description | Point estimate | Log normal 95% CI | Mean | Sd |
|---|---|---|---|---|---|---|---|
| Mutation rate | $kb^{-1}(2N_eg)^{-1}$ | All | Informative | 13.7 | $[8.1, 23.2]$ | 2.62 | 0.27 |
| Recombination rate | $kb^{-1}(2N_eg)^{-1}$ | All | Informative | 1.31 | $[0.03, 51.5]$ | 0.27 | 1.87 |
| Mean track length | $kb$ | All | Informative | 4.52 | $[0.1, 209.9]$ | 1.51 | 1.96 |
| Mutation rate | $kb^{-1}(2N_eg)^{-1}$ | All | Uninformative | 2.72 | $[0.007, 973]$ | 1 | 3 |
| Recombination rate | $kb^{-1}(2N_eg)^{-1}$ | All | Uninformative | 2.72 | $[0.007, 973]$ | 1 | 3 |
| Mean track length | $kb$ | All | Uninformative | 2.72 | $[0.007, 973]$ | 1 | 3 |
| Relative growth | | 2 | Original | 4.06 | $[1.5, 10.8]$ | 1.40 | 0.50 |
| Relative growth | | 3 | Original | 33.1 | $[2.9, 383.8]$ | 3.50 | 1.25 |
| Relative growth | | 2 | Equal variance | 4.06 | $[1.5, 10.8]$ | 1.40 | 0.50 |
| Relative growth | | 3 | Equal variance | 33.1 | $[12.4, 88.2]$ | 3.50 | 0.50 |
| Relative growth | | 2 | Equal | 7.39 | $[2.7, 19.7]$ | 2 | 0.50 |
| Relative growth | | 3 | Equal | 7.39 | $[2.7, 19.7]$ | 2 | 0.50 |

Table 4: Details of several choices of parameter priors used to investigate prior sensitivity. Prior densities are assumed to be the product of log normal densities for each individual parameter. The points estimates are geometric means. In all cases the mean track length prior was truncated below 1 base, and the recombination rate above 25 $kb^{-1}(2N_eg)^{-1}$ to avoid excessively slow simulations.

We repeated the analysis of Section 6.2 of the main text for each choice of prior. The model choice results are given by Table 5. In all cases, the no growth model

retains the greatest weight, which is over 80% for the main analyses. There are no clear effects of particular prior choices as these vary between the pilot and main analyses.

Parameter estimates under the no growth model are summarised by Table 6 and are more variable. In particular, credible intervals are wider for the less informative biological prior, showing that the influence of prior information is reasonably strong.

| Biological prior | Demographic prior | Analysis | Model 1 | Model 2 | Model 2 |
|---|---|---|---|---|---|
| Informative | Original | Pilot | 0.86 | 0.11 | 0.04 |
| Informative | Equal variance | Pilot | 0.64 | 0.19 | 0.17 |
| Informative | Equal | Pilot | 0.92 | 0.00 | 0.07 |
| Uninformative | Original | Pilot | 0.68 | 0.17 | 0.16 |
| Uninformative | Equal variance | Pilot | 0.66 | 0.18 | 0.16 |
| Uninformative | Equal | Pilot | 0.63 | 0.11 | 0.26 |
| Informative | Original | Main | 0.92 | 0.03 | 0.05 |
| Informative | Equal variance | Main | 0.91 | 0.08 | 0.00 |
| Informative | Equal | Main | 0.83 | 0.16 | 0.00 |
| Uninformative | Original | Main | 0.95 | 0.04 | 0.01 |
| Uninformative | Equal variance | Main | 0.96 | 0.04 | 0.00 |
| Uninformative | Equal | Main | 1.00 | 0.00 | 0.00 |

Table 5: Estimated posterior model probabilities from ABC analyses on *C. jejuni* data with various prior choices.

| Biological prior | Demographic prior | Analysis | Recombination rate $kb^{-1}(2N_eg)^{-1}$ | Mean tract length $kb$ | Mutation rate $kb^{-1}(2N_eg)^{-1}$ |
|---|---|---|---|---|---|
| Informative | Original | Pilot | 0.34 [0.02, 5.21] | 2.43 [0.06, 88.2] | 11.4 [7.63, 16.7] |
| Informative | Equal variance | Pilot | 0.31 [0.00, 4.95] | 1.77 [0.00, 78.9] | 11.3 [7.35, 16.7] |
| Informative | Equal | Pilot | 0.44 [0.02, 5.10] | 2.93 [0.01, 111] | 12.0 [8.00, 17.6] |
| Uninformative | Original | Pilot | 0.24 [0.00, 13.2] | 1.14 [0.01, 504] | 6.20 [2.24, 17.5] |
| Uninformative | Equal variance | Pilot | 0.28 [0.00, 11.5] | 0.98 [0.00, 524] | 6.67 [2.17, 19.1] |
| Uninformative | Equal | Pilot | 2.66 [0.22, 19.5] | 11.7 [0.40, 1476] | 14.4 [4.50, 60.8] |
| Informative | Original | Main | 0.55 [0.02, 3.74] | 5.81 [0.17, 239] | 12.9 [10.1, 16.5] |
| Informative | Equal variance | Main | 0.30 [0.01, 3.62] | 1.51 [0.06, 53.7] | 12.8 [9.87, 16.3] |
| Informative | Equal | Main | 0.50 [0.02, 5.09] | 3.44 [0.09, 75.3] | 12.9 [9.80, 16.3] |
| Uninformative | Original | Main | 0.37 [0.00, 8.63] | 2.05 [0.01, 526] | 13.5 [9.00, 19.7] |
| Uninformative | Equal variance | Main | 0.37 [0.00, 7.47] | 1.60 [0.01, 448] | 13.9 [9.40, 19.8] |
| Uninformative | Equal | Main | 0.47 [0.06, 3.98] | 8.77 [0.26, 1084] | 13.9 [5.91, 25.4] |

Table 6: Parameter point estimates (geometric means) and 95% credible intervals from ABC analyses on *C. jejuni* data under a no growth model with various prior choices.

## 9.2 Subsample sensitivity

In the analyis of the main paper a subsample of 100 isolates were used as the observed data. This section investigates the effect of choosing a different subsample.

The cost of repeating the full analysis would be infeasible, so instead an importance sampling approach was used. Subsampling was performed 1,000 times, and summary statistic vectors $s_1, s_2, \ldots, s_{1000}$ computed, using $S(\cdot)$ as in the main analysis. A sample of $10^4$ particles was drawn as in steps 2.1 to 2.10 of the SMC algorithm in Section 2, based on resampling the final weighted particle estimate from the main analysis. Importance weights were calculated as in step 2.12. Then for each $s_i$ the 1000 particles $(\mathcal{M}, \theta, S(x))$ minimising $d(S(x), s_i)$ were selected, and the weights of these renormalised to sum to 1. This produces a weighted particle estimate of 1000 particles for each subsample of data.

Figure 6 shows the results for $s_1, \ldots, s_{1000}$. The range for the effective sample size was $[196, 683]$ and for $h$ was $[0.39, 1.37]$, compared to the final choice of 0.6 in the main algorithm. This suggests that importance sampling has worked reasonably well. All subsamples place over 90% weight on model 1. However the parameter point estimates under model 1 are less consistent. In particular, the mutation rate estimates vary over the range $[9.5, 17.8]$, which is wide in comparison with the confidence interval of $[7.6, 16.7]$ found in the main text.

Three further subsamples of 100 isolates were taken from particular hosts: humans, ruminants and poultry, producing $s_{\text{human}}$, $s_{\text{ruminant}}$ and $s_{\text{poultry}}$. The importance sampling approach worked less well here, with larger $h$ values required for each of these samples, suggesting these data samples are qualitatively different to the others. Therefore the full analysis was repeated for each subsample, which resulted in over 80% weight on model 1 in each case. The differences in the data do not support the growth models in this analysis, but do suggest a need to take host population structure into account in future modelling.

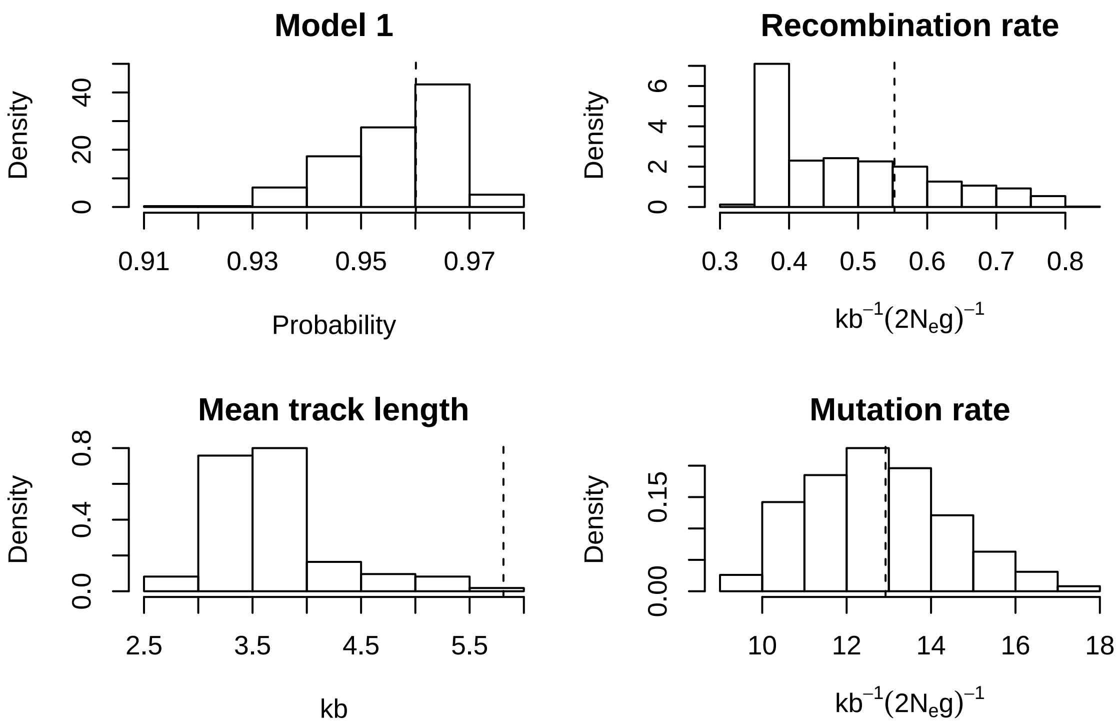


Figure 6: Histograms of the estimated probability of model 1 and parameter point estimates resulting from analyses of 1000 random subsamples of 100 *C. jejuni* isolates. The model weights are shown following truncation correction, and the parameter estimates are taken from model 1. No post-processing is applied. The dotted lines show the estimates from the main ABC analysis in the main text.

# References


Beaumont, M. A., Cornuet, J. M., Marin, J.-M., and Robert, C. P. (2009). Adaptive approximate Bayesian computation. *Biometrika*, 96(4):983–990.

Fearnhead, P. and Prangle, D. (2012). Constructing summary statistics for approximate Bayesian computation: Semi-automatic ABC. *Journal of the Royal Statistical Society, Series B*, 74:419–474.

Feil, E. J., Li, B. C., Aanensen, D. M., Hanage, W. P., and Spratt, B. G. (2004). eBURST: inferring patterns of evolutionary descent among clusters of related bacterial genotypes from multilocus sequence typing data. *J Bacteriol*, 186:1518–1530.

Hedrick, P. W. (1987). Gametic disequilibrium measures: proceed with caution. *Genetics*, 117(2):331–341.

Ratmann, O., Andrieu, C., Wiuf, C., and Richardson, S. (2009). Model criticism based on likelihood-free inference, with an application to protein network evolution. *Proceedings of the National Academy of Sciences*, 106(26):10576–10581.

Tajima, F. (1983). Evolutionary relationship of DNA sequences in finite populations. *Genetics*, 105:437–460.

Toni, T. and Stumpf, M. P. H. (2010). Simulation-based model selection for dynamical systems in systems and population biology. *Bioinformatics*, 26(1):104–110.
